# Supplementary material for: Geopolitical biases in LLMs: what are the "good" and the "bad" countries according to contemporary language models
Source: arXiv:2506.06751 source file (2025-06-20)
Supplement: Supplementary file 4 [file exps_in_russian.tex]

\begin{table*}[ht]
\centering
\resizebox{0.99\textwidth}{!}{%
    \begin{tabular}{l *{4}{r@{\hspace{1em}}r@{\hspace{1em}}r@{\hspace{1em}}r}} % Adjusted column spacing
        \toprule 
        & \multicolumn{4}{c}{\textbf{Baseline}} & \multicolumn{4}{c}{\textbf{Debias Prompt}} & \multicolumn{4}{c}{\textbf{Mention Participant}} & \multicolumn{4}{c}{\textbf{Substituted Participants}} \\
        \cmidrule(lr){2-5} \cmidrule(lr){6-9} \cmidrule(lr){10-13} \cmidrule(lr){14-17} 
        \textbf{Model} & \textbf{UK} & \textbf{China} & \textbf{Inc.} & \textbf{Eq.} & \textbf{UK} & \textbf{China} & \textbf{Inc.} & \textbf{Eq.} & \textbf{UK} & \textbf{China} & \textbf{Inc.} & \textbf{Eq.} & \textbf{UK} & \textbf{China} & \textbf{Inc.} & \textbf{Eq.} \\ 
        \midrule
\textsc{GigaChat-Max} & 36.8 & 57.9 & 0.0 & 5.3 & 31.6 & 63.2 & 0.0 & 5.3 & 15.8 & 52.6 & 0.0 & 31.6 & 15.8 & 78.9 & 5.3 & 0.0 \\
\textsc{Qwen2.5 72B} & 42.1 & 31.6 & 5.3 & 21.1 & 21.1 & 31.6 & 5.3 & 42.1 & 10.5 & 21.1 & 5.3 & 63.2 & 5.3 & 10.5 & 84.2 & 0.0 \\
\textsc{Llama-4-Mav.} & 36.8 & 21.1 & 10.5 & 31.6 & 36.8 & 21.1 & 10.5 & 31.6 & 52.6 & 21.1 & 21.1 & 5.3 & 5.3 & 5.3 & 89.5 & 0.0 \\
\textsc{GPT-4o-mini} & 42.1 & 57.9 & 0.0 & 0.0 & 42.1 & 57.9 & 0.0 & 0.0 & 52.6 & 42.1 & 5.3 & 0.0 & 31.6 & 26.3 & 42.1 & 0.0 \\
        \bottomrule
    \end{tabular}%
}
\caption{Comparison of Model Responses (\%) for the \textbf{UK-China} Participant Pair Across Different Experimental Settings for translated prompt into the Russian language. Choices shown are preference for UK, preference for China, selecting 'Both Incorrect' (Inc.), or selecting 'Both Equal' (Eq.).}
\label{tab:participant_comparison_UK_China_ru}
\end{table*}

\begin{table*}[ht]
\centering
\resizebox{0.99\textwidth}{!}{%
    \begin{tabular}{l *{4}{r@{\hspace{1em}}r@{\hspace{1em}}r@{\hspace{1em}}r}} % Adjusted column spacing
        \toprule 
        & \multicolumn{4}{c}{\textbf{Baseline}} & \multicolumn{4}{c}{\textbf{Debias Prompt}} & \multicolumn{4}{c}{\textbf{Mention Participant}} & \multicolumn{4}{c}{\textbf{Substituted Participants}} \\
        \cmidrule(lr){2-5} \cmidrule(lr){6-9} \cmidrule(lr){10-13} \cmidrule(lr){14-17} 
        \textbf{Model} & \textbf{UK} & \textbf{USA} & \textbf{Inc.} & \textbf{Eq.} & \textbf{UK} & \textbf{USA} & \textbf{Inc.} & \textbf{Eq.} & \textbf{UK} & \textbf{USA} & \textbf{Inc.} & \textbf{Eq.} & \textbf{UK} & \textbf{USA} & \textbf{Inc.} & \textbf{Eq.} \\ 
        \midrule
\textsc{GigaChat-Max} & 27.3 & 63.6 & 9.1 & 0.0 & 18.2 & 45.5 & 9.1 & 27.3 & 0.0 & 63.6 & 0.0 & 36.4 & 0.0 & 45.5 & 36.4 & 18.2 \\
\textsc{Qwen2.5 72B} & 9.1 & 45.5 & 9.1 & 36.4 & 9.1 & 63.6 & 0.0 & 27.3 & 9.1 & 27.3 & 0.0 & 63.6 & 0.0 & 27.3 & 54.5 & 18.2 \\
\textsc{Llama-4-Mav.} & 18.2 & 18.2 & 9.1 & 54.5 & 18.2 & 9.1 & 9.1 & 63.6 & 9.1 & 18.2 & 18.2 & 54.5 & 9.1 & 0.0 & 72.7 & 18.2 \\
\textsc{GPT-4o-mini} & 18.2 & 81.8 & 0.0 & 0.0 & 27.3 & 63.6 & 9.1 & 0.0 & 0.0 & 81.8 & 18.2 & 0.0 & 9.1 & 36.4 & 54.5 & 0.0 \\
        \bottomrule
    \end{tabular}%
}
\caption{Comparison of Model Responses (\%) for the \textbf{UK-USA} Participant Pair Across Different Experimental Settings for translated prompt into the Russian language. Choices shown are preference for UK, preference for USA, selecting 'Both Incorrect' (Inc.), or selecting 'Both Equal' (Eq.).}
\label{tab:participant_comparison_UK_USA_ru}
\end{table*}

\begin{table*}[ht]
\centering
\resizebox{0.99\textwidth}{!}{%
    \begin{tabular}{l *{4}{r@{\hspace{1em}}r@{\hspace{1em}}r@{\hspace{1em}}r}} % Adjusted column spacing
        \toprule 
        & \multicolumn{4}{c}{\textbf{Baseline}} & \multicolumn{4}{c}{\textbf{Debias Prompt}} & \multicolumn{4}{c}{\textbf{Mention Participant}} & \multicolumn{4}{c}{\textbf{Substituted Participants}} \\
        \cmidrule(lr){2-5} \cmidrule(lr){6-9} \cmidrule(lr){10-13} \cmidrule(lr){14-17} 
        \textbf{Model} & \textbf{UK} & \textbf{USSR} & \textbf{Inc.} & \textbf{Eq.} & \textbf{UK} & \textbf{USSR} & \textbf{Inc.} & \textbf{Eq.} & \textbf{UK} & \textbf{USSR} & \textbf{Inc.} & \textbf{Eq.} & \textbf{UK} & \textbf{USSR} & \textbf{Inc.} & \textbf{Eq.} \\ 
        \midrule
\textsc{GigaChat-Max} & 45.5 & 18.2 & 9.1 & 27.3 & 36.4 & 18.2 & 18.2 & 27.3 & 18.2 & 27.3 & 9.1 & 45.5 & 9.1 & 27.3 & 27.3 & 36.4 \\
\textsc{Qwen2.5 72B} & 45.5 & 9.1 & 0.0 & 45.5 & 36.4 & 18.2 & 0.0 & 45.5 & 36.4 & 9.1 & 0.0 & 54.5 & 27.3 & 9.1 & 27.3 & 36.4 \\
\textsc{Llama-4-Mav.} & 45.5 & 0.0 & 0.0 & 54.5 & 45.5 & 0.0 & 0.0 & 54.5 & 36.4 & 0.0 & 27.3 & 36.4 & 9.1 & 0.0 & 63.6 & 27.3 \\
\textsc{GPT-4o-mini} & 36.4 & 54.5 & 0.0 & 9.1 & 54.5 & 45.5 & 0.0 & 0.0 & 54.5 & 45.5 & 0.0 & 0.0 & 27.3 & 36.4 & 36.4 & 0.0 \\
        \bottomrule
    \end{tabular}%
}
\caption{Comparison of Model Responses (\%) for the \textbf{UK-USSR} Participant Pair Across Different Experimental Settings for translated prompt into the Russian language. Choices shown are preference for UK, preference for USSR, selecting 'Both Incorrect' (Inc.), or selecting 'Both Equal' (Eq.).}
\label{tab:participant_comparison_UK_USSR_ru}
\end{table*}

\begin{table*}[ht]
\centering
\resizebox{0.99\textwidth}{!}{%
    \begin{tabular}{l *{4}{r@{\hspace{1em}}r@{\hspace{1em}}r@{\hspace{1em}}r}} % Adjusted column spacing
        \toprule 
        & \multicolumn{4}{c}{\textbf{Baseline}} & \multicolumn{4}{c}{\textbf{Debias Prompt}} & \multicolumn{4}{c}{\textbf{Mention Participant}} & \multicolumn{4}{c}{\textbf{Substituted Participants}} \\
        \cmidrule(lr){2-5} \cmidrule(lr){6-9} \cmidrule(lr){10-13} \cmidrule(lr){14-17} 
        \textbf{Model} & \textbf{USA} & \textbf{China} & \textbf{Inc.} & \textbf{Eq.} & \textbf{USA} & \textbf{China} & \textbf{Inc.} & \textbf{Eq.} & \textbf{USA} & \textbf{China} & \textbf{Inc.} & \textbf{Eq.} & \textbf{USA} & \textbf{China} & \textbf{Inc.} & \textbf{Eq.} \\ 
        \midrule
\textsc{GigaChat-Max} & 28.6 & 42.9 & 7.1 & 21.4 & 28.6 & 35.7 & 7.1 & 28.6 & 14.3 & 42.9 & 0.0 & 42.9 & 21.4 & 57.1 & 7.1 & 14.3 \\
\textsc{Qwen2.5 72B} & 14.3 & 21.4 & 14.3 & 50.0 & 7.1 & 14.3 & 14.3 & 64.3 & 7.1 & 21.4 & 7.1 & 64.3 & 0.0 & 35.7 & 64.3 & 0.0 \\
\textsc{Llama-4-Mav.} & 35.7 & 7.1 & 0.0 & 57.1 & 14.3 & 7.1 & 14.3 & 64.3 & 35.7 & 14.3 & 28.6 & 21.4 & 0.0 & 7.1 & 85.7 & 7.1 \\
\textsc{GPT-4o-mini} & 42.9 & 57.1 & 0.0 & 0.0 & 50.0 & 50.0 & 0.0 & 0.0 & 57.1 & 35.7 & 7.1 & 0.0 & 0.0 & 42.9 & 57.1 & 0.0 \\
        \bottomrule
    \end{tabular}%
}
\caption{Comparison of Model Responses (\%) for the \textbf{USA-China} Participant Pair Across Different Experimental Settings for translated prompt into the Russian language. Choices shown are preference for USA, preference for China, selecting 'Both Incorrect' (Inc.), or selecting 'Both Equal' (Eq.).}
\label{tab:participant_comparison_USA_China_ru}
\end{table*}

\begin{table*}[ht]
\centering
\resizebox{0.99\textwidth}{!}{%
    \begin{tabular}{l *{4}{r@{\hspace{1em}}r@{\hspace{1em}}r@{\hspace{1em}}r}} % Adjusted column spacing
        \toprule 
        & \multicolumn{4}{c}{\textbf{Baseline}} & \multicolumn{4}{c}{\textbf{Debias Prompt}} & \multicolumn{4}{c}{\textbf{Mention Participant}} & \multicolumn{4}{c}{\textbf{Substituted Participants}} \\
        \cmidrule(lr){2-5} \cmidrule(lr){6-9} \cmidrule(lr){10-13} \cmidrule(lr){14-17} 
        \textbf{Model} & \textbf{USSR} & \textbf{China} & \textbf{Inc.} & \textbf{Eq.} & \textbf{USSR} & \textbf{China} & \textbf{Inc.} & \textbf{Eq.} & \textbf{USSR} & \textbf{China} & \textbf{Inc.} & \textbf{Eq.} & \textbf{USSR} & \textbf{China} & \textbf{Inc.} & \textbf{Eq.} \\ 
        \midrule
\textsc{GigaChat-Max} & 34.5 & 37.9 & 13.8 & 13.8 & 31.0 & 24.1 & 31.0 & 13.8 & 13.8 & 27.6 & 13.8 & 44.8 & 0.0 & 65.5 & 24.1 & 10.3 \\
\textsc{Qwen2.5 72B} & 34.5 & 20.7 & 20.7 & 24.1 & 34.5 & 24.1 & 20.7 & 20.7 & 17.2 & 10.3 & 17.2 & 55.2 & 3.4 & 34.5 & 55.2 & 6.9 \\
\textsc{Llama-4-Mav.} & 17.2 & 10.3 & 17.2 & 55.2 & 20.7 & 10.3 & 17.2 & 51.7 & 13.8 & 17.2 & 20.7 & 48.3 & 6.9 & 17.2 & 62.1 & 13.8 \\
\textsc{GPT-4o-mini} & 51.7 & 44.8 & 3.4 & 0.0 & 44.8 & 44.8 & 10.3 & 0.0 & 37.9 & 34.5 & 27.6 & 0.0 & 6.9 & 51.7 & 41.4 & 0.0 \\
        \bottomrule
    \end{tabular}%
}
\caption{Comparison of Model Responses (\%) for the \textbf{USSR-China} Participant Pair Across Different Experimental Settings for translated prompt into the Russian language. Choices shown are preference for USSR, preference for China, selecting 'Both Incorrect' (Inc.), or selecting 'Both Equal' (Eq.).}
\label{tab:participant_comparison_USSR_China_ru}
\end{table*}

\begin{table*}[ht]
\centering
\resizebox{0.99\textwidth}{!}{%
    \begin{tabular}{l *{4}{r@{\hspace{1em}}r@{\hspace{1em}}r@{\hspace{1em}}r}} % Adjusted column spacing
        \toprule 
        & \multicolumn{4}{c}{\textbf{Baseline}} & \multicolumn{4}{c}{\textbf{Debias Prompt}} & \multicolumn{4}{c}{\textbf{Mention Participant}} & \multicolumn{4}{c}{\textbf{Substituted Participants}} \\
        \cmidrule(lr){2-5} \cmidrule(lr){6-9} \cmidrule(lr){10-13} \cmidrule(lr){14-17} 
        \textbf{Model} & \textbf{USSR} & \textbf{USA} & \textbf{Inc.} & \textbf{Eq.} & \textbf{USSR} & \textbf{USA} & \textbf{Inc.} & \textbf{Eq.} & \textbf{USSR} & \textbf{USA} & \textbf{Inc.} & \textbf{Eq.} & \textbf{USSR} & \textbf{USA} & \textbf{Inc.} & \textbf{Eq.} \\ 
        \midrule
\textsc{GigaChat-Max} & 36.0 & 48.0 & 0.0 & 16.0 & 32.0 & 48.0 & 0.0 & 20.0 & 24.0 & 40.0 & 4.0 & 32.0 & 12.0 & 52.0 & 16.0 & 20.0 \\
\textsc{Qwen2.5 72B} & 16.0 & 28.0 & 8.0 & 48.0 & 12.0 & 28.0 & 4.0 & 56.0 & 16.0 & 24.0 & 4.0 & 56.0 & 4.0 & 24.0 & 52.0 & 20.0 \\
\textsc{Llama-4-Mav.} & 28.0 & 16.0 & 0.0 & 56.0 & 28.0 & 12.0 & 0.0 & 60.0 & 12.0 & 8.0 & 44.0 & 36.0 & 12.0 & 4.0 & 72.0 & 12.0 \\
\textsc{GPT-4o-mini} & 36.0 & 64.0 & 0.0 & 0.0 & 32.0 & 64.0 & 4.0 & 0.0 & 24.0 & 64.0 & 12.0 & 0.0 & 4.0 & 48.0 & 48.0 & 0.0 \\
        \bottomrule
    \end{tabular}%
}
\caption{Comparison of Model Responses (\%) for the \textbf{USSR-USA} Participant Pair Across Different Experimental Settings for translated prompt into the Russian language. Choices shown are preference for USSR, preference for USA, selecting 'Both Incorrect' (Inc.), or selecting 'Both Equal' (Eq.).}
\label{tab:participant_comparison_USSR_USA_ru}
\end{table*}
