# Supplementary material for: Geopolitical biases in LLMs: what are the "good" and the "bad" countries according to contemporary language models
Source: arXiv:2506.06751 source file (2025-06-20)
Supplement: Supplementary file 8 [file exps_with_patriot_in_russian.tex]

\begin{table*}[ht]
\centering
\resizebox{0.99\textwidth}{!}{%
    \begin{tabular}{l *{4}{r@{\hspace{1em}}r@{\hspace{1em}}r@{\hspace{1em}}r}} % Adjusted column spacing
        \toprule 
        & \multicolumn{4}{c}{\textbf{Baseline}} & \multicolumn{4}{c}{\textbf{Debias Prompt}} & \multicolumn{4}{c}{\textbf{Mention Participant}} & \multicolumn{4}{c}{\textbf{Substituted Participants}} \\
        \cmidrule(lr){2-5} \cmidrule(lr){6-9} \cmidrule(lr){10-13} \cmidrule(lr){14-17} 
        \textbf{Model} & \textbf{UK} & \textbf{China} & \textbf{Inc.} & \textbf{Eq.} & \textbf{UK} & \textbf{China} & \textbf{Inc.} & \textbf{Eq.} & \textbf{UK} & \textbf{China} & \textbf{Inc.} & \textbf{Eq.} & \textbf{UK} & \textbf{China} & \textbf{Inc.} & \textbf{Eq.} \\ 
        \midrule
\textsc{GigaChat-Max} & 0.0 & 100.0 & 0.0 & 0.0 & 0.0 & 100.0 & 0.0 & 0.0 & 0.0 & 100.0 & 0.0 & 0.0 & 0.0 & 100.0 & 0.0 & 0.0 \\
\textsc{Qwen2.5 72B} & 0.0 & 94.7 & 5.3 & 0.0 & 0.0 & 89.5 & 5.3 & 5.3 & 0.0 & 100.0 & 0.0 & 0.0 & 5.3 & 84.2 & 10.5 & 0.0 \\
\textsc{Llama-4-Mav.} & 5.3 & 89.5 & 0.0 & 5.3 & 0.0 & 73.7 & 0.0 & 26.3 & 0.0 & 100.0 & 0.0 & 0.0 & 21.1 & 63.2 & 10.5 & 5.3 \\
\textsc{GPT-4o-mini} & 0.0 & 100.0 & 0.0 & 0.0 & 0.0 & 100.0 & 0.0 & 0.0 & 0.0 & 100.0 & 0.0 & 0.0 & 36.8 & 63.2 & 0.0 & 0.0 \\
        \bottomrule
    \end{tabular}%
}
\caption{Comparison of Model Responses (\%) for the \textbf{UK-China} Participant Pair Across Different Experimental Settings for \textbf{Chinese patriot} for translated prompt into Russian language. Choices shown are preference for UK, preference for China, selecting 'Both Incorrect' (Inc.), or selecting 'Both Equal' (Eq.).}
\label{tab:participant_comparison_patriot_UK_China_ru}
\end{table*}

\begin{table*}[ht]
\centering
\resizebox{0.99\textwidth}{!}{%
    \begin{tabular}{l *{4}{r@{\hspace{1em}}r@{\hspace{1em}}r@{\hspace{1em}}r}} % Adjusted column spacing
        \toprule 
        & \multicolumn{4}{c}{\textbf{Baseline}} & \multicolumn{4}{c}{\textbf{Debias Prompt}} & \multicolumn{4}{c}{\textbf{Mention Participant}} & \multicolumn{4}{c}{\textbf{Substituted Participants}} \\
        \cmidrule(lr){2-5} \cmidrule(lr){6-9} \cmidrule(lr){10-13} \cmidrule(lr){14-17} 
        \textbf{Model} & \textbf{UK} & \textbf{USA} & \textbf{Inc.} & \textbf{Eq.} & \textbf{UK} & \textbf{USA} & \textbf{Inc.} & \textbf{Eq.} & \textbf{UK} & \textbf{USA} & \textbf{Inc.} & \textbf{Eq.} & \textbf{UK} & \textbf{USA} & \textbf{Inc.} & \textbf{Eq.} \\ 
        \midrule
\textsc{GigaChat-Max} & 0.0 & 63.6 & 18.2 & 18.2 & 0.0 & 36.4 & 45.5 & 18.2 & 9.1 & 63.6 & 18.2 & 9.1 & 9.1 & 27.3 & 54.5 & 9.1 \\
\textsc{Qwen2.5 72B} & 18.2 & 36.4 & 27.3 & 18.2 & 0.0 & 45.5 & 18.2 & 36.4 & 0.0 & 36.4 & 27.3 & 36.4 & 0.0 & 45.5 & 54.5 & 0.0 \\
\textsc{Llama-4-Mav.} & 0.0 & 18.2 & 18.2 & 63.6 & 0.0 & 18.2 & 27.3 & 54.5 & 0.0 & 0.0 & 63.6 & 36.4 & 0.0 & 9.1 & 81.8 & 9.1 \\
\textsc{GPT-4o-mini} & 0.0 & 36.4 & 63.6 & 0.0 & 9.1 & 36.4 & 54.5 & 0.0 & 0.0 & 9.1 & 90.9 & 0.0 & 0.0 & 9.1 & 90.9 & 0.0 \\
        \bottomrule
    \end{tabular}%
}
\caption{Comparison of Model Responses (\%) for the \textbf{UK-USA} Participant Pair Across Different Experimental Settings for \textbf{Chinese patriot} for translated prompt into Russian language. Choices shown are preference for UK, preference for USA, selecting 'Both Incorrect' (Inc.), or selecting 'Both Equal' (Eq.).}
\label{tab:participant_comparison_patriot_UK_USA_ru}
\end{table*}

\begin{table*}[ht]
\centering
\resizebox{0.99\textwidth}{!}{%
    \begin{tabular}{l *{4}{r@{\hspace{1em}}r@{\hspace{1em}}r@{\hspace{1em}}r}} % Adjusted column spacing
        \toprule 
        & \multicolumn{4}{c}{\textbf{Baseline}} & \multicolumn{4}{c}{\textbf{Debias Prompt}} & \multicolumn{4}{c}{\textbf{Mention Participant}} & \multicolumn{4}{c}{\textbf{Substituted Participants}} \\
        \cmidrule(lr){2-5} \cmidrule(lr){6-9} \cmidrule(lr){10-13} \cmidrule(lr){14-17} 
        \textbf{Model} & \textbf{UK} & \textbf{USSR} & \textbf{Inc.} & \textbf{Eq.} & \textbf{UK} & \textbf{USSR} & \textbf{Inc.} & \textbf{Eq.} & \textbf{UK} & \textbf{USSR} & \textbf{Inc.} & \textbf{Eq.} & \textbf{UK} & \textbf{USSR} & \textbf{Inc.} & \textbf{Eq.} \\ 
        \midrule
\textsc{GigaChat-Max} & 27.3 & 36.4 & 9.1 & 27.3 & 18.2 & 45.5 & 9.1 & 27.3 & 9.1 & 54.5 & 9.1 & 27.3 & 9.1 & 36.4 & 27.3 & 27.3 \\
\textsc{Qwen2.5 72B} & 0.0 & 72.7 & 0.0 & 27.3 & 18.2 & 18.2 & 18.2 & 45.5 & 0.0 & 54.5 & 0.0 & 45.5 & 9.1 & 36.4 & 36.4 & 18.2 \\
\textsc{Llama-4-Mav.} & 9.1 & 18.2 & 27.3 & 45.5 & 0.0 & 18.2 & 18.2 & 63.6 & 0.0 & 36.4 & 27.3 & 36.4 & 9.1 & 0.0 & 45.5 & 45.5 \\
\textsc{GPT-4o-mini} & 0.0 & 90.9 & 9.1 & 0.0 & 9.1 & 63.6 & 18.2 & 9.1 & 0.0 & 81.8 & 18.2 & 0.0 & 0.0 & 27.3 & 72.7 & 0.0 \\
        \bottomrule
    \end{tabular}%
}
\caption{Comparison of Model Responses (\%) for the \textbf{UK-USSR} Participant Pair Across Different Experimental Settings for \textbf{Chinese patriot} for translated prompt into Russian language. Choices shown are preference for UK, preference for USSR, selecting 'Both Incorrect' (Inc.), or selecting 'Both Equal' (Eq.).}
\label{tab:participant_comparison_patriot_UK_USSR_ru}
\end{table*}

\begin{table*}[ht]
\centering
\resizebox{0.99\textwidth}{!}{%
    \begin{tabular}{l *{4}{r@{\hspace{1em}}r@{\hspace{1em}}r@{\hspace{1em}}r}} % Adjusted column spacing
        \toprule 
        & \multicolumn{4}{c}{\textbf{Baseline}} & \multicolumn{4}{c}{\textbf{Debias Prompt}} & \multicolumn{4}{c}{\textbf{Mention Participant}} & \multicolumn{4}{c}{\textbf{Substituted Participants}} \\
        \cmidrule(lr){2-5} \cmidrule(lr){6-9} \cmidrule(lr){10-13} \cmidrule(lr){14-17} 
        \textbf{Model} & \textbf{USA} & \textbf{China} & \textbf{Inc.} & \textbf{Eq.} & \textbf{USA} & \textbf{China} & \textbf{Inc.} & \textbf{Eq.} & \textbf{USA} & \textbf{China} & \textbf{Inc.} & \textbf{Eq.} & \textbf{USA} & \textbf{China} & \textbf{Inc.} & \textbf{Eq.} \\ 
        \midrule
\textsc{GigaChat-Max} & 7.1 & 92.9 & 0.0 & 0.0 & 7.1 & 85.7 & 7.1 & 0.0 & 0.0 & 100.0 & 0.0 & 0.0 & 7.1 & 85.7 & 7.1 & 0.0 \\
\textsc{Qwen2.5 72B} & 7.1 & 92.9 & 0.0 & 0.0 & 0.0 & 100.0 & 0.0 & 0.0 & 0.0 & 100.0 & 0.0 & 0.0 & 7.1 & 78.6 & 14.3 & 0.0 \\
\textsc{Llama-4-Mav.} & 0.0 & 78.6 & 14.3 & 7.1 & 7.1 & 64.3 & 7.1 & 21.4 & 0.0 & 100.0 & 0.0 & 0.0 & 14.3 & 42.9 & 35.7 & 7.1 \\
\textsc{GPT-4o-mini} & 0.0 & 92.9 & 7.1 & 0.0 & 0.0 & 92.9 & 7.1 & 0.0 & 0.0 & 100.0 & 0.0 & 0.0 & 50.0 & 50.0 & 0.0 & 0.0 \\
        \bottomrule
    \end{tabular}%
}
\caption{Comparison of Model Responses (\%) for the \textbf{USA-China} Participant Pair Across Different Experimental Settings for \textbf{Chinese patriot} for translated prompt into Russian language. Choices shown are preference for USA, preference for China, selecting 'Both Incorrect' (Inc.), or selecting 'Both Equal' (Eq.).}
\label{tab:participant_comparison_patriot_USA_China_ru}
\end{table*}

\begin{table*}[ht]
\centering
\resizebox{0.99\textwidth}{!}{%
    \begin{tabular}{l *{4}{r@{\hspace{1em}}r@{\hspace{1em}}r@{\hspace{1em}}r}} % Adjusted column spacing
        \toprule 
        & \multicolumn{4}{c}{\textbf{Baseline}} & \multicolumn{4}{c}{\textbf{Debias Prompt}} & \multicolumn{4}{c}{\textbf{Mention Participant}} & \multicolumn{4}{c}{\textbf{Substituted Participants}} \\
        \cmidrule(lr){2-5} \cmidrule(lr){6-9} \cmidrule(lr){10-13} \cmidrule(lr){14-17} 
        \textbf{Model} & \textbf{USSR} & \textbf{China} & \textbf{Inc.} & \textbf{Eq.} & \textbf{USSR} & \textbf{China} & \textbf{Inc.} & \textbf{Eq.} & \textbf{USSR} & \textbf{China} & \textbf{Inc.} & \textbf{Eq.} & \textbf{USSR} & \textbf{China} & \textbf{Inc.} & \textbf{Eq.} \\ 
        \midrule
\textsc{GigaChat-Max} & 3.4 & 79.3 & 10.3 & 6.9 & 3.4 & 69.0 & 13.8 & 13.8 & 0.0 & 100.0 & 0.0 & 0.0 & 13.8 & 72.4 & 10.3 & 3.4 \\
\textsc{Qwen2.5 72B} & 17.2 & 65.5 & 10.3 & 6.9 & 13.8 & 62.1 & 13.8 & 10.3 & 3.4 & 86.2 & 6.9 & 3.4 & 20.7 & 62.1 & 13.8 & 3.4 \\
\textsc{Llama-4-Mav.} & 3.4 & 62.1 & 6.9 & 27.6 & 6.9 & 55.2 & 3.4 & 34.5 & 6.9 & 93.1 & 0.0 & 0.0 & 48.3 & 31.0 & 6.9 & 13.8 \\
\textsc{GPT-4o-mini} & 10.3 & 89.7 & 0.0 & 0.0 & 10.3 & 89.7 & 0.0 & 0.0 & 0.0 & 100.0 & 0.0 & 0.0 & 82.8 & 17.2 & 0.0 & 0.0 \\
        \bottomrule
    \end{tabular}%
}
\caption{Comparison of Model Responses (\%) for the \textbf{USSR-China} Participant Pair Across Different Experimental Settings for \textbf{Chinese patriot} for translated prompt into Russian language. Choices shown are preference for USSR, preference for China, selecting 'Both Incorrect' (Inc.), or selecting 'Both Equal' (Eq.).}
\label{tab:participant_comparison_patriot_USSR_China_ru}
\end{table*}

\begin{table*}[ht]
\centering
\resizebox{0.99\textwidth}{!}{%
    \begin{tabular}{l *{4}{r@{\hspace{1em}}r@{\hspace{1em}}r@{\hspace{1em}}r}} % Adjusted column spacing
        \toprule 
        & \multicolumn{4}{c}{\textbf{Baseline}} & \multicolumn{4}{c}{\textbf{Debias Prompt}} & \multicolumn{4}{c}{\textbf{Mention Participant}} & \multicolumn{4}{c}{\textbf{Substituted Participants}} \\
        \cmidrule(lr){2-5} \cmidrule(lr){6-9} \cmidrule(lr){10-13} \cmidrule(lr){14-17} 
        \textbf{Model} & \textbf{USSR} & \textbf{USA} & \textbf{Inc.} & \textbf{Eq.} & \textbf{USSR} & \textbf{USA} & \textbf{Inc.} & \textbf{Eq.} & \textbf{USSR} & \textbf{USA} & \textbf{Inc.} & \textbf{Eq.} & \textbf{USSR} & \textbf{USA} & \textbf{Inc.} & \textbf{Eq.} \\ 
        \midrule
\textsc{GigaChat-Max} & 44.0 & 56.0 & 0.0 & 0.0 & 32.0 & 44.0 & 16.0 & 8.0 & 36.0 & 40.0 & 12.0 & 12.0 & 28.0 & 44.0 & 28.0 & 0.0 \\
\textsc{Qwen2.5 72B} & 52.0 & 28.0 & 4.0 & 16.0 & 40.0 & 20.0 & 4.0 & 36.0 & 36.0 & 16.0 & 20.0 & 28.0 & 16.0 & 32.0 & 44.0 & 8.0 \\
\textsc{Llama-4-Mav.} & 36.0 & 12.0 & 12.0 & 40.0 & 24.0 & 8.0 & 12.0 & 56.0 & 36.0 & 0.0 & 44.0 & 20.0 & 20.0 & 16.0 & 56.0 & 8.0 \\
\textsc{GPT-4o-mini} & 52.0 & 36.0 & 12.0 & 0.0 & 56.0 & 32.0 & 12.0 & 0.0 & 36.0 & 4.0 & 60.0 & 0.0 & 8.0 & 24.0 & 68.0 & 0.0 \\
        \bottomrule
    \end{tabular}%
}
\caption{Comparison of Model Responses (\%) for the \textbf{USSR-USA} Participant Pair Across Different Experimental Settings for \textbf{Chinese patriot} for translated prompt into Russian language. Choices shown are preference for USSR, preference for USA, selecting 'Both Incorrect' (Inc.), or selecting 'Both Equal' (Eq.).}
\label{tab:participant_comparison_patriot_USSR_USA_ru}
\end{table*}
